# Supplementary material for: Generalized Benders Decomposition with Continual Learning for Hybrid Model Predictive Control in Dynamic Environment
Source: arXiv:2310.03344 source file (2023-10-10)
Supplement: Supplementary file 1 [file appendix_proof_of_lemma_3.tex]

The following lemma is an effort to quantify how shifted cutting planes benefit by removing infeasible contact sequences. However, it is still vague and the bound may not be too good. We also need good dual gap for it to be valid. Maybe the right way to use it is to only investigate the beginning iteration.

\begin{definition}
(Shifted mode sequence) Let a sequence of binary variables $\boldsymbol{z} \in \mathbb{R}^{Nn_{z}}$ be $\boldsymbol{z} = [\boldsymbol{z}_{0}, \ \boldsymbol{z}_{1}, ..., \ \boldsymbol{z}_{N-1}]$. We define a shifted mode sequence as $\boldsymbol{z}_s = [\boldsymbol{z}_{1}, \ \boldsymbol{z}_{2}, ..., \ \boldsymbol{z}_{N-1}, \ast] \in \mathbb{R}^{Nn_{z}}$ where $\ast$ denotes any possible $\boldsymbol{z}_{N} \in \mathbb{R}^{n_{z}}$.
\end{definition}

\xuan{If shifted contact sequence is defined, then why is this approach better than shifted contact sequence as warm-start?}

\begin{lemma}
Assume a sequence $\boldsymbol{z}$ is infeasible for the subproblem ~\eqref{Eqn:subproblem_MLD} under given $\boldsymbol{x}_{ini}$. Then the shifted $\boldsymbol{z}_s$ is: 
\begin{enumerate}
    \item Infeasible for ~\eqref{Eqn:subproblem_MLD} under given $\boldsymbol{x}_{ini}$ if $\boldsymbol{x}_{ini}^T(\tilde{\nu}_{1} - \tilde{\nu}_{0}) - b(\boldsymbol{z}_0)^T\tilde{\nu}_{1} - d(\boldsymbol{z}_0)^T\tilde{\lambda}_{0} \leq 0$ \xuan{(Make this condition independent of $\boldsymbol\lambda$ so it only depends on $\boldsymbol{x}_{ini}$ and $\boldsymbol{z}$! Is $\boldsymbol\lambda$ unique?)}.
    \item Does not violate the existing feasibility cuts (in particular, ~\eqref{Eqn:feasible_cutting_plane}) under conditions xxx.
    \item Its optimality evaluated at $\boldsymbol{z}_{s}$ of the existing optimality cuts ~\eqref{Eqn:optimal_cut_MLD} is at most higher than its evaluation at $\boldsymbol{z}$ by $v(\boldsymbol{x}_{ini}, \tilde{\boldsymbol{z}}_i) - (v(\boldsymbol{x}_{ini}, \tilde{\boldsymbol{z}}_{i,s})-v(\boldsymbol{x}_{1}, \tilde{\boldsymbol{z}}_i)) + ||\boldsymbol\nu_{0}^*|| \  ||\boldsymbol{x}_{ini} - \boldsymbol{x}_1|| + ||\boldsymbol\nu^{*}|| \ ||\boldsymbol{b}(\boldsymbol{0}, \Delta\boldsymbol{z})|| + ||\boldsymbol\lambda^{*}|| \ ||\boldsymbol{d}(\Delta\boldsymbol{z})||$ \xuan{Notation is chaotic here!}.
\end{enumerate}
\label{Lem:lemma3}
\end{lemma}

\begin{proof}
To prove the infeasibility of $\boldsymbol{z}_s$, we can construct Farkas certificate. Since $\boldsymbol{z}$ is infeasible, there exists $\tilde{\boldsymbol\nu} \in \mathbb{R}^{(N+1)n_{x}}$, $\tilde{\boldsymbol\lambda} \in \mathbb{R}^{Nn_{c}}$ satisfying ~\eqref{Eqn:Farkas_proof}. Expand ~\eqref{Eqn:Farkas_proof}, we have:

\begin{subequations}
\begin{align}
    i=0,..., N-1, \ \ \tilde{\boldsymbol\lambda}_i &\geq \boldsymbol{0} \label{Eqn:infeasible_cond_1} \\
    i=0,..., N-1, \ \ \bar{\boldsymbol{I}}^T \tilde{\boldsymbol\nu}_{i} + \bar{\boldsymbol{J}}^T \tilde{\boldsymbol\nu}_{i+1} + \boldsymbol{d}^T \tilde{\boldsymbol\lambda}_i &= \boldsymbol{0} \label{Eqn:infeasible_cond_2} \\
    \boldsymbol{I}_{n_x} \tilde{\boldsymbol\nu}_{N} &= \boldsymbol{0} \label{Eqn:infeasible_cond_3} \\
    \boldsymbol{x}_{ini}^T \tilde{\boldsymbol\nu}_{0} + \sum_{i=1}^{N} \boldsymbol{b}^T(\boldsymbol{z}_{i-1}) \tilde{\boldsymbol\nu}_{i} + \sum_{j=0}^{N-1} \boldsymbol{d}(\boldsymbol{z}_{j})^T \tilde{\boldsymbol\lambda}_{j} &< 0 \label{Eqn:infeasible_cond_4}    
\end{align}
\end{subequations}

Where $\tilde{\boldsymbol\lambda}_i$, $\tilde{\boldsymbol\nu}_{i}$ correspond to the infeasible certificates $\tilde{\boldsymbol\lambda}$ and $\tilde{\boldsymbol\nu}$ at time step $i$. Define the shifted infeasible certificate:

\begin{equation}
\begin{aligned}
    \tilde{\boldsymbol\lambda}_{s} = [\tilde{\boldsymbol\lambda}_{1}^T, \tilde{\boldsymbol\lambda}_{2}^T, ..., \tilde{\boldsymbol\lambda}_{N-1}^T, \boldsymbol{0}_{n_c}^T]^T \ \in \mathbb{R}^{Nn_{c}} \\
    \tilde{\boldsymbol\nu}_{s} = [\tilde{\boldsymbol\nu}_{1}^T, \tilde{\boldsymbol\nu}_{2}^T, ..., \tilde{\boldsymbol\nu}_{N}^T, \boldsymbol{0}_{n_x}^T]^T \ \in \mathbb{R}^{(N+1)n_{x}}
\end{aligned}
\end{equation}

It is easy to verify that the shifted infeasible certificates satisfy ~\eqref{Eqn:infeasible_cond_1}, ~\eqref{Eqn:infeasible_cond_2}, ~\eqref{Eqn:infeasible_cond_3}. If $\boldsymbol{x}_{ini}^T(\tilde{\nu}_{1} - \tilde{\nu}_{0}) - b(\boldsymbol{z}_0)^T\tilde{\nu}_{1} - d(\boldsymbol{z}_0)^T\tilde{\lambda}_{0} \leq 0$ is also true, we have

\begin{equation}
    \boldsymbol{x}_{ini}^T \tilde{\boldsymbol\nu}_{s,0} + \sum_{i=1}^{N} \boldsymbol{b}^T(\boldsymbol{z}_{s,i-1}) \tilde{\boldsymbol\nu}_{E,i} + \sum_{j=0}^{N-1} \boldsymbol{d}(\boldsymbol{z}_{s,j})^T \tilde{\boldsymbol\lambda}_{s,j} < 0
\end{equation}

Hence $\boldsymbol{z}_s$ is infeasible for the subproblem ~\eqref{Eqn:subproblem_MLD} under given $\boldsymbol{x}_{ini}$. Note that $\boldsymbol{z}_s$ does not violate the original cutting plane ~\eqref{Eqn:Farkas_proof} under certain condition. We will show this at the end.

To investigate the optimality. We first show that the shifted problem decreases the cost by certain amount. Define the shifted problem:

\begin{equation}
\begin{aligned}
   v(\boldsymbol{x}_{1}, \boldsymbol{z}) =  \underset{\boldsymbol{x} \in X}{\text{minimize}} \ \ & \sum_{k=0}^{N-1} \boldsymbol{x}_{k}^{T} \boldsymbol{Q} \boldsymbol{x}_{k} + \boldsymbol{x}_{N}^{T} \boldsymbol{Q}_{N} \boldsymbol{x}_{N}\\
    \text{s.t.} \ \ & \boldsymbol{A} \boldsymbol{x} = \boldsymbol{b}(\boldsymbol{x}_{1}, \boldsymbol{z})\\
    & \boldsymbol{C} \boldsymbol{x} \leq \boldsymbol{d}(\boldsymbol{z})
\end{aligned}
\end{equation}

Where $\boldsymbol{x}_{1} = \boldsymbol{A} \boldsymbol{x}_{ini} + \boldsymbol{B} \boldsymbol{u}_0^* + \boldsymbol{b}(\boldsymbol{z}_0^*)$. Show that the optimal $\boldsymbol{z}$ is also shifted $\boldsymbol{z}_s$. Show that the objective function decreases by a certain amount $v(\boldsymbol{x}_{1}, \boldsymbol{z})-v(\boldsymbol{x}_{ini}, \boldsymbol{z}_s)$ \xuan{Nonuniform Q may cause some trouble here!}.

Write out the cutting plane for the shifted problem:

\begin{equation}
    v(\boldsymbol{x}_{1}, \boldsymbol{z}_s) = \underset{\boldsymbol\nu, \boldsymbol\lambda \geq \boldsymbol{0}}{\text{maximize}} \ \ \underset{\boldsymbol{x} \in X}{\text{minimize}} \ \ \mathcal{L}(\boldsymbol{x}, \boldsymbol\nu, \boldsymbol\lambda; \boldsymbol{x}_{1}, \boldsymbol{z}_s)
\end{equation}

However, we will use the dual varaibles from the original problem $(\boldsymbol{x}_{ini}, \boldsymbol{z})$ instead of the shifted problem, since they are both dual feasible. This means weak duality:

\begin{equation}
    v(\boldsymbol{x}_{1}, \boldsymbol{z}_s) \geq \underset{\boldsymbol{x} \in X}{\text{minimize}} \ \ \mathcal{L}(\boldsymbol{x}, \boldsymbol\nu^*, \boldsymbol\lambda^*; \boldsymbol{x}_{1}, \boldsymbol{z}_s)
\end{equation}

As the unconstrained minimizer $\boldsymbol{x}^0$ does not depend on $(\boldsymbol{x}_{1}, \boldsymbol{z}_s)$ but depend on $(\boldsymbol\nu^*, \boldsymbol\lambda^*)$, they are shared with the problem $(\boldsymbol{x}_{ini}, \boldsymbol{z})$. Therefore, the cutting plane is: \xuan{The form of cutting plane is a little confusing. Consider still use the original form, but write simplified form in summary parts.}

\begin{equation}
\begin{aligned}
    \mathcal{L}(\boldsymbol{x}^0, \boldsymbol\nu, \boldsymbol\lambda; \boldsymbol{x}_{1}, \boldsymbol{z}_s) = f_{obj}(\boldsymbol{x}^0) &+ \boldsymbol\nu^{*T} \boldsymbol{A} \boldsymbol{x}^0 - \boldsymbol\nu^{*T} \boldsymbol{b}(\boldsymbol{x}_{1}, \boldsymbol{z}_s) \\
    &+ \boldsymbol\lambda^{*T} \boldsymbol{C}^0 \boldsymbol{x}^0 - \boldsymbol\lambda^{*T} \boldsymbol{d}(\boldsymbol{z}_s)
\end{aligned}
\end{equation}

Since $\boldsymbol{x}^0$ is shared with the problem $(\boldsymbol{x}_{ini}, \boldsymbol{z})$, the only difference of this cutting plane with optimality cut $(\boldsymbol{x}_{ini}, \boldsymbol{z}_s)$ is the $\boldsymbol{x}_1$ term (cutting plane $(\boldsymbol{x}_{ini}, \boldsymbol{z}_s)$ has $\boldsymbol{x}_{ini}$). We can bound this term using Cauchy-Schwartz inequality. The difference is:

\begin{equation}
    ||\boldsymbol\nu_{0}^{*T} (\boldsymbol{x}_{ini} - \boldsymbol{x}_1)|| \leq ||\boldsymbol\nu_{0}^*|| \  ||\boldsymbol{x}_{ini} - \boldsymbol{x}_1||
\end{equation}

Therefore, the cutting plane with $(\boldsymbol{x}_{ini}, \boldsymbol{z}_s)$ is lower than $(\boldsymbol{x}_{ini}, \boldsymbol{z})$ with a difference:

\begin{equation}
\begin{aligned}
    v(\boldsymbol{x}_{ini}, \boldsymbol{z}_s) \leq v(\boldsymbol{x}_{ini}, \boldsymbol{z}) &- (v(\boldsymbol{x}_{ini}, \boldsymbol{z}_s)-v(\boldsymbol{x}_{1}, \boldsymbol{z})) \\
    &+ ||\boldsymbol\nu_{0}^*|| \  ||\boldsymbol{x}_{ini} - \boldsymbol{x}_1||
\end{aligned}
\end{equation}

We then look at how the value of this cutting plane changes by shifting $\boldsymbol{z}^{\prime}$ that is not $\boldsymbol{z}$. This can be gauged by looking at the similarity of $\boldsymbol{z}^{\prime}$ and $\boldsymbol{z}$. Let $C(\boldsymbol{x}^0, \boldsymbol\nu^{*}, \boldsymbol\lambda^{*}) = f_{obj}(\boldsymbol{x}^0) + \boldsymbol\nu^{*T} \boldsymbol{A} \boldsymbol{x}^0 + \boldsymbol\lambda^{*T} \boldsymbol{C}\boldsymbol{x}^0$.

\begin{equation}
\begin{aligned}
    &C(\boldsymbol{x}^0, \boldsymbol\nu^{*}, \boldsymbol\lambda^{*}) - \boldsymbol\nu^{*T} \boldsymbol{b}(\boldsymbol{x}_{ini}, \boldsymbol{z}^{\prime}_s) - \boldsymbol\lambda^{*T} \boldsymbol{d}(\boldsymbol{z}^{\prime}_s) \\
    = \ &C(\boldsymbol{x}^0, \boldsymbol\nu^{*}, \boldsymbol\lambda^{*}) - \boldsymbol\nu^{*T} \boldsymbol{b}(\boldsymbol{x}_{ini}, \boldsymbol{z}_s) - \boldsymbol\lambda^{*T} \boldsymbol{d}(\boldsymbol{z}_s) \\
    + \ &\boldsymbol\nu^{*T} (\boldsymbol{b}(\boldsymbol{x}_{ini}, \boldsymbol{z}_s) - \boldsymbol{b}(\boldsymbol{x}_{ini}, \boldsymbol{z}^{\prime}_s)) + \boldsymbol\lambda^{*T}(\boldsymbol{d}(\boldsymbol{z}_s) - \boldsymbol{d}(\boldsymbol{z}^{\prime}_s))
\end{aligned}
\end{equation}

The first term is just cutting plane $(\boldsymbol{x}_{ini}, \boldsymbol{z}_s)$. The second term can be bounded using Cauchy-Schwartz inequality:

\begin{equation}
\begin{aligned}
    ||\boldsymbol\nu^{*T} (\boldsymbol{b}(\boldsymbol{x}_{ini}, \boldsymbol{z}_s) - &\boldsymbol{b}(\boldsymbol{x}_{ini}, \boldsymbol{z}^{\prime}_s))|| \\
    &\leq ||\boldsymbol\nu^{*}|| \ ||\boldsymbol{b}(\boldsymbol{x}_{ini}, \boldsymbol{z}_s) - \boldsymbol{b}(\boldsymbol{x}_{ini}, \boldsymbol{z}^{\prime}_s)|| \\
    ||\boldsymbol\lambda^{*T}(\boldsymbol{d}(\boldsymbol{z}_s) - \boldsymbol{d}(\boldsymbol{z}^{\prime}_s))|| &\leq ||\boldsymbol\lambda^{*}|| \ ||\boldsymbol{d}(\boldsymbol{z}_s) - \boldsymbol{d}(\boldsymbol{z}^{\prime}_s)||
\end{aligned}
\end{equation}

If $\boldsymbol{b}$ and $\boldsymbol{d}$ are linear, the differences are: $||\boldsymbol{b}(\boldsymbol{0}, \boldsymbol{z}_s-\boldsymbol{z}^{\prime}_s))||$, $||\boldsymbol{d}(\boldsymbol{z}_s - \boldsymbol{z}^{\prime}_s)||$.

\xuan{You may have forgotten the d($\ast$).}

To prove that $\boldsymbol{z}_s$ does not violate the original cutting plane ~\eqref{Eqn:Farkas_proof}, if $\boldsymbol \lambda$ is unique, you can define a feasible problem using the infeasible $\boldsymbol \lambda$ to build the optimality cut, and re-use the proof above to show this cut is looser after shifting.
\end{proof}

\xuan{This lemma is still vague and does not clearly convey an idea of how to add/not add this shifted cut. Although those bounds look awkward, you should study when they can be used so we don't need to add all the cuts. Maybe it will benefit presolve. When are the cuts active, and can we use it to solve MIP?}

Lemma \ref{Lem:lemma3} gives a bound of the value of the optimality cuts by shifting the current choice of $\boldsymbol{z}$. This result says that the shifted mode sequence may appear to be fairly optimal depending on the similarity of $\boldsymbol{z}$ with their generating $\tilde{\boldsymbol{z}}_i$, despite that it is in fact infeasible. In fact, if $\Delta\boldsymbol{z}=\boldsymbol{0}$ and the $\boldsymbol{x}_{ini}$ term is smaller than the difference of cost, $\boldsymbol{z}_s$ is a more optimal solution for this cut $i$. Since the master problem is seeking more optimal solutions according to the lower bounds, adding shifted cutting planes saves iterations for the master problem to explore $\boldsymbol{z}_s$.
