# Supplementary material for: Generalized Benders Decomposition with Continual Learning for Hybrid Model Predictive Control in Dynamic Environment
Source: arXiv:2310.03344 source file (2023-10-10)
Supplement: Supplementary file 2 [file appendix_rank_deficient.tex]

Since $\bar{\boldsymbol{Q}}$ and $\boldsymbol{Q}_{N}$ are assumed to be positive semi-definite, they can be diagonalized using orthogonal transformation $\hat{\boldsymbol{Q}} = \boldsymbol{T}^{-1} \bar{\boldsymbol{Q}} \boldsymbol{T}$, $\hat{\boldsymbol{Q}}_N = \boldsymbol{T}^{-1} \bar{\boldsymbol{Q}}_N \boldsymbol{T}$. $\hat{\boldsymbol{Q}}$, $\hat{\boldsymbol{Q}}_N$ are diagonal matrices. With a coordinate transform, the $\bar{\boldsymbol{x}}$ related terms become $\sum_{k=0}^{N-1} \tilde{\boldsymbol{x}}_{k}^{T} \hat{\boldsymbol{Q}} \tilde{\boldsymbol{x}}_{k} + \tilde{\boldsymbol{x}}_{N}^{T} \hat{\boldsymbol{Q}}_{N} \tilde{\boldsymbol{x}}_{N} + \boldsymbol\lambda_{E}^T\tilde{\boldsymbol{A}}\tilde{\boldsymbol{x}} + \boldsymbol\lambda_{I}^T\tilde{\boldsymbol{C}}\tilde{\boldsymbol{x}}$. When taking first order derivatives, the corresponding $\tilde{\boldsymbol{x}}$ should satisfy $\sum_{i} \boldsymbol\lambda_{E}^T[i]\tilde{\boldsymbol{A}}[i,j] + \sum_{i} \boldsymbol\lambda_{I}^T[i]\tilde{\boldsymbol{C}}[i,j] =0$. This guarantees the inner minimization to be bounded, and eliminates the need to add additional constraints as Tobia did. When constructing optimal cutting planes, we use $\boldsymbol\lambda_{E}^*, \boldsymbol\lambda_{I}^*$ returned from the solver. \xuan{This condition needs to be invariant under parameters. How do you guarantee they satisfy the conditions? If Q is not diagonal, there may be issue!!}
